# Supplementary material for: Enhancing the Generalization for Intent Classification and Out-of-Domain Detection in SLU
Source: arXiv:2106.14464 source file (2021-06-28)
Supplement: Supplementary file 1 [file math.tex]

\section{Mathematical Hypothesis and Explanation of OOD Overconfidence}\label{ap:math}

Let $f^c$ be the unnormalized probability $\widehat{p}(\ry |\vx)$ and $f^d$ be the unnormalized probability $\widehat{p}(\rd=1|\vx)$,
i.e., $\widehat{p}(\ry |\vx) = \textsl{norm}(f^c(\vx))$, $\widehat{p}(\rd=1 |\vx) = \textsl{norm}(f^d(\vx))$.
We call the unnormalized probability ``logits".
We hypothesize the following:
\begin{equation}\label{eq:hyp}
    \textsl{norm}\Big({f^c(\vx) \over f^d(\vx)}\Big) \propto {\textsl{norm}(f^c(\vx)) \over \textsl{norm}(f^d(\vx))}
\end{equation}

Then, we mathematically explain the overconfidence phenomena observed in \citep{overconfidence17} given the assumption in~\autoref{eq:hyp}.
First, we can rewrite \autoref{eq:dis_posterior} as follows:
\begin{eqnarray*}
& \widehat{p}(\ry|\rd=1, \vx) &
\approx \frac{\widehat{p}(\ry |\vx)}{\widehat{p}(\rd=1|\vx)}
= {\textsl{norm}(f^c(\vx)) \over \textsl{norm}(f^d(\vx))} \\
&&\propto \textsl{norm}\Big({f^c(\vx) \over f^d(\vx)}\Big)
\end{eqnarray*}

Then, we use the following ``softmax function"~\citep{Goodfellow2016DL} to normalize the logits to be a probability distribution:
\begin{eqnarray*}
& \widehat{p}(\ry|\rd=1, \vx) &
\propto \textsl{softmax}\Big({f^c(\vx) \over f^d(\vx)}\Big) \\
&& = \frac{\textsl{exp}(\frac{f^c_i(\vx)}{f^d_i(\vx)})}{\sum_{j=1}^C{\textsl{exp}(\frac{f^c_j(\vx)}{f^d_j(\vx)})}}
\end{eqnarray*}

\begin{figure}[h]
	\centering
	\includegraphics[width=0.7\columnwidth]{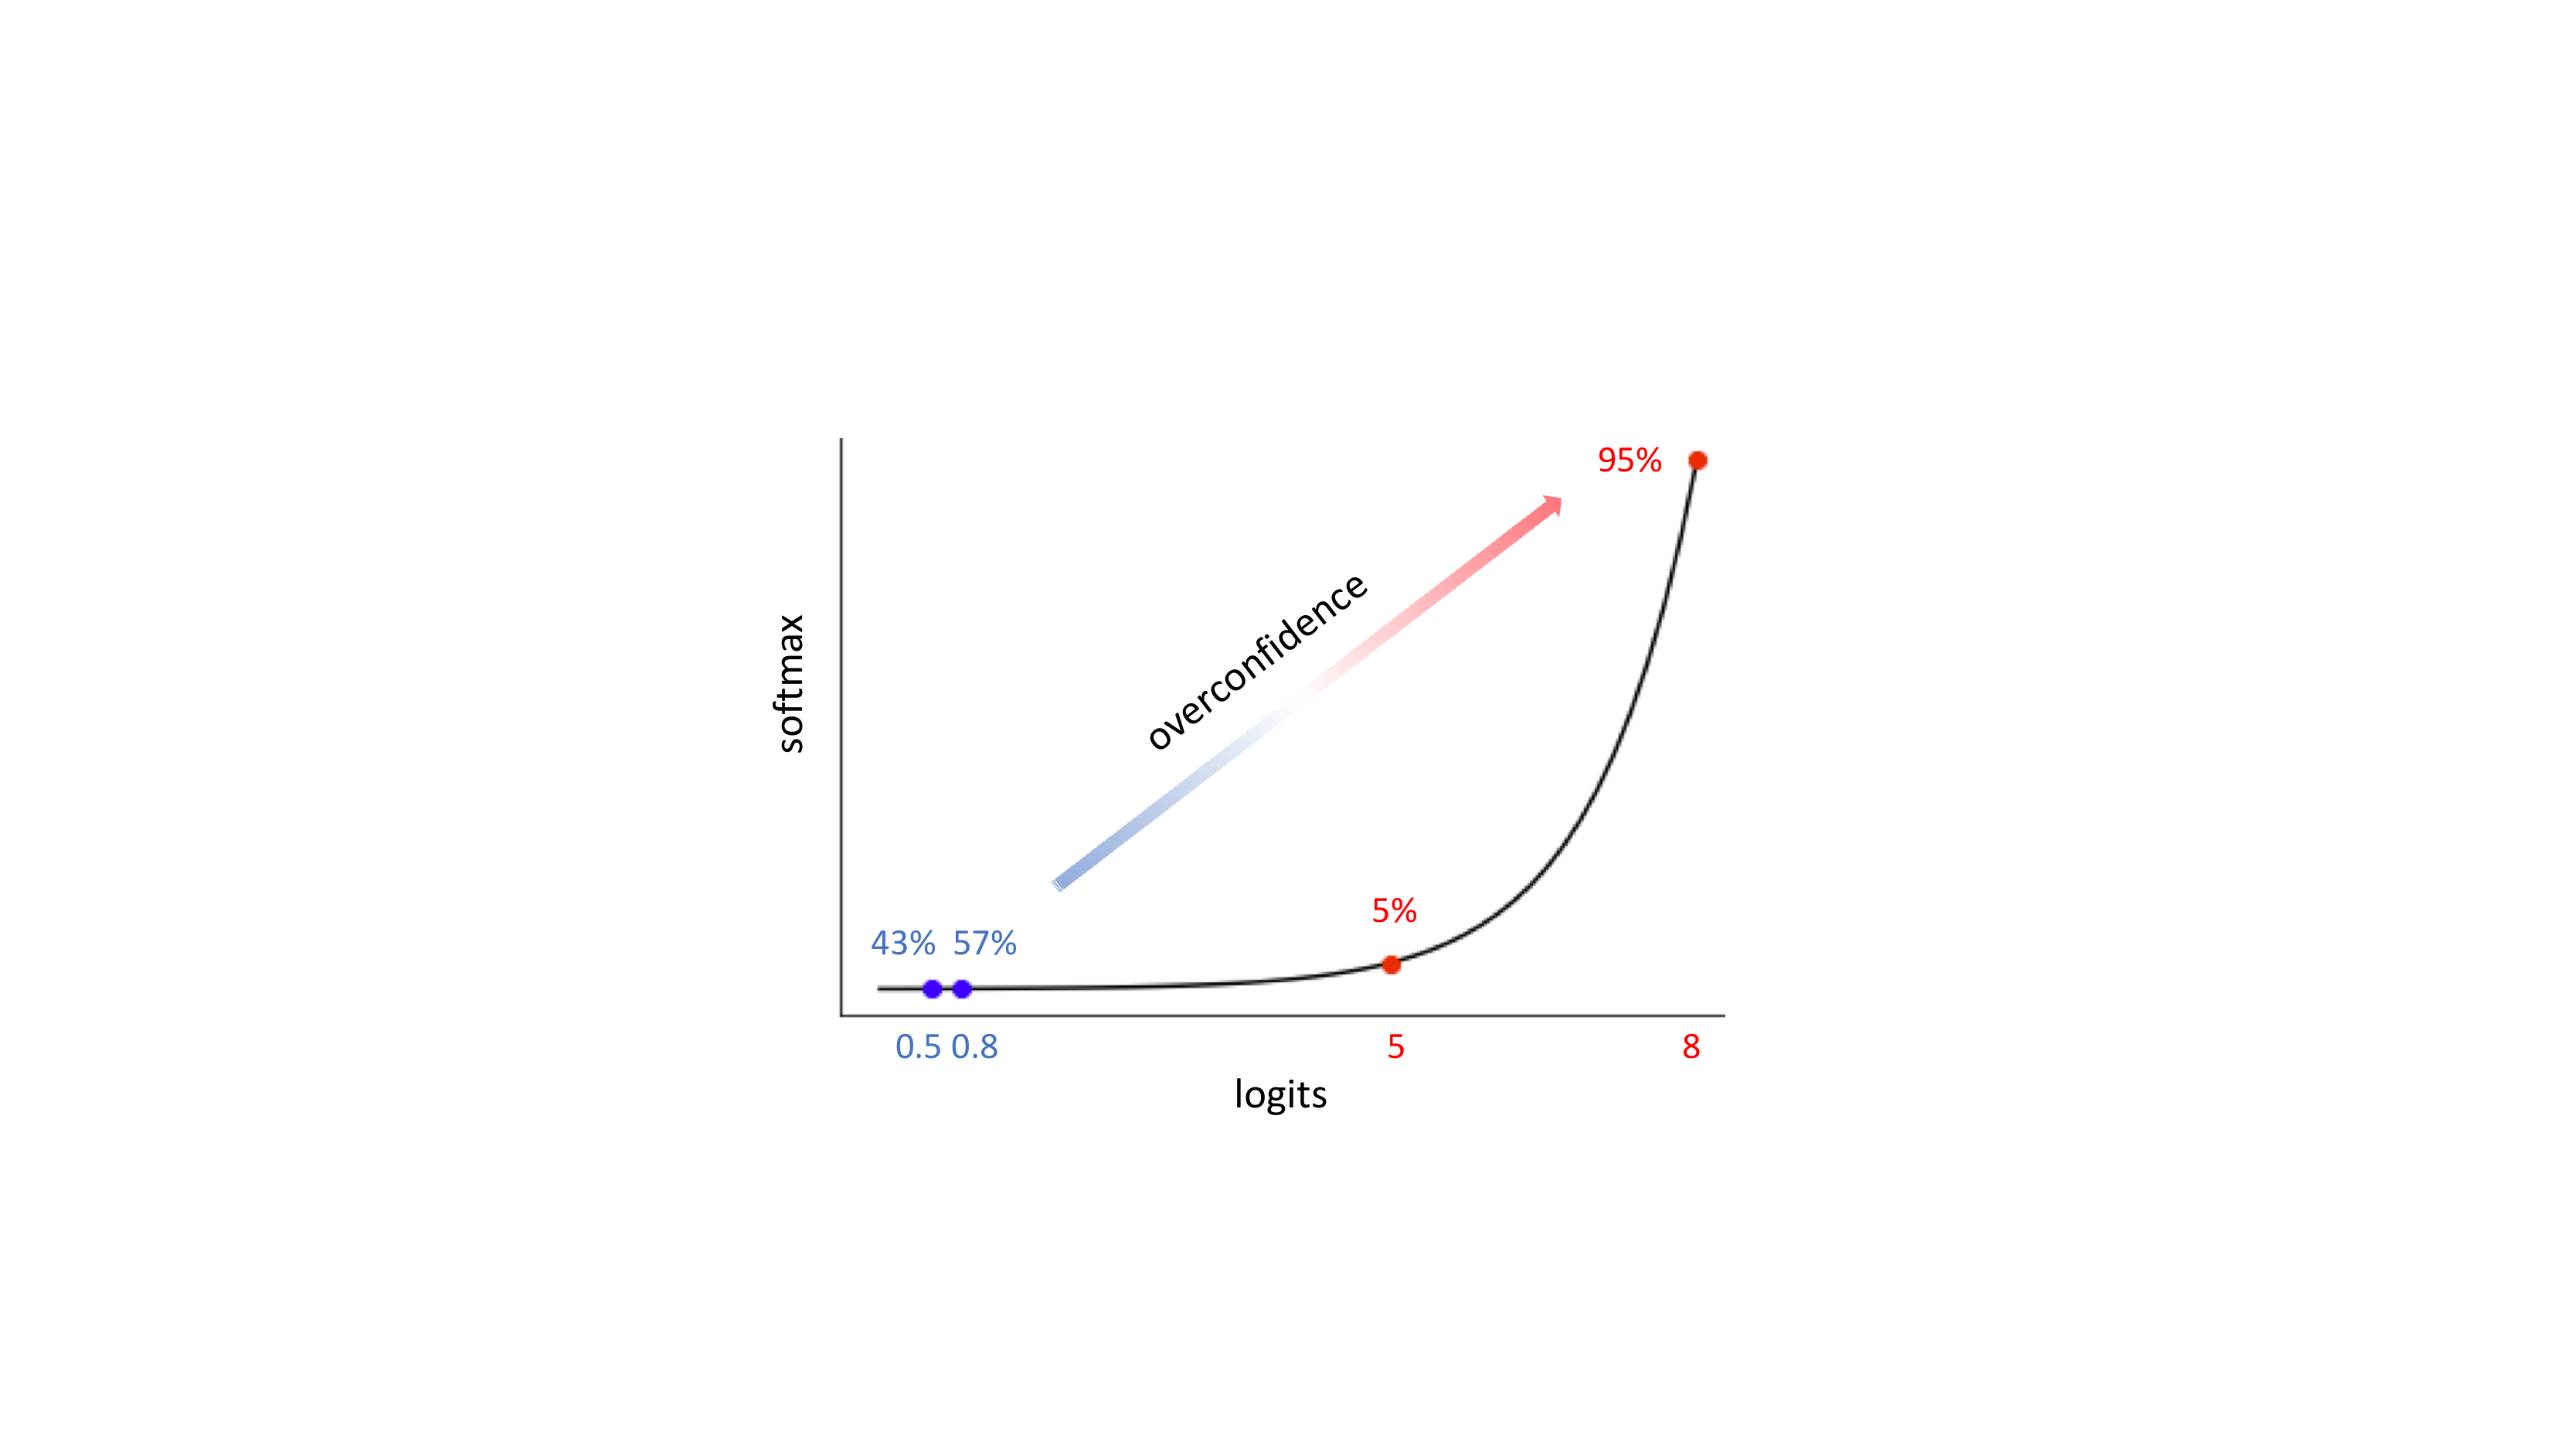}
	\caption{Overconfidence Explanation for an Out-of-Domain Utterance}
	\label{fig:overconfidence}
\end{figure}

We illustrate our overconfidence explanation in~\autoref{fig:overconfidence} using an example:
Assuming there are two in-domain classes in our classifier.  For an out-of-domain $\vx$, it is expected that $f_c(\vx)$ (the unnormalized $\widehat{p}(\ry| \vx)$) (blue points in Figure \ref{fig:overconfidence}) for both classes are small, e.g., 0.5 and 0.8.
The normalization function maps $f_c(\vx)$ to probabilities 43\% and 57\%.
However, for an out-of-domain $\vx$, $f_d(\vx)$ ((the unnormalized $\widehat{p}(\rd=1|\vx)$) is a very small number, e.g., 0.1.
After $f_c(\vx)$ is divided by the small $f_d(\vx)$, the final model logits (red points in~\autoref{fig:overconfidence}) for both classes become 5 and 8.
The softmax normalization maps them to probabilities 5\% and 95\%.
With that, the model will conclude that $\vx$ is classified into class \#2 with a confidence level of 95\%. This shows how a wrong decision can be made with overconfidence for out-of-domain utterance.
