# Supplementary material for: Enhancing the Generalization for Intent Classification and Out-of-Domain Detection in SLU
Source: arXiv:2106.14464 source file (2021-06-28)
Supplement: Supplementary file 4 [file implementation.tex]

\section{Implementation and Training Details}

We implemented our model using PyTorch on top of the Hugging Face transformer library \citep{Wolf2019HuggingFacesTS}.
Since our model does not have additional hyperparamters, we simply follow all the hyperparameters in original models.
To avoid overfitting, we apply early stop during model training \citep{Goodfellow2016DL}.
% We use the model with the IND intent classification accuracy reaches 99.5\% of the best accuracy on validation set by tracking the accuracy.
For the above datasets, thanks to the pretrained BERT based models, the training phase takes only 1-3 epochs.
We conducted experiments on two transformer based architectures, BERT \citep{devlin2018bert} and RoBERTa \citep{Liu2019roberta}.
All experiments are run on GPU Tesla M40.
